# Supplementary material for: Convolutional neural networks for long-time dissipative quantum dynamics
Source: arXiv:2012.11009 source file (2020-12-20)
Supplement: Supplementary file 1 [file si.pdf]

Supporting Information for:

# Convolutional neural networks for long-time dissipative quantum dynamics

Luis E. Herrera Rodríguez[1, 2, 3] and Alexei A. Kananenka[3]

[1] *Departamento de Física, Universidad Nacional de Colombia, Carrera 30 No. 45-03, Bogotá D.C., Colombia*
[2] *Escuela de Ciencias Básicas, Tecnología e Ingeniería, Universidad Nacional Abierta y a Distancia, Facatativá, Colombia*
[3] *Department of Physics and Astronomy, University of Delaware, Newark, DE 19711, USA*

TABLE S1. Parameters of the plots shown in Figures S1-S5. The common parameters are the electronic coupling $J = 100$ cm$^{-1}$ and the cut-off frequency $\omega_c = 53$ cm$^{-1}$. See main text for details.

| Subfigure | $\Delta$ [cm$^{-1}$] | $\lambda$ [cm$^{-1}$] | $T$ [K] | Subfigure | $\Delta$ [cm$^{-1}$] | $\lambda$ [cm$^{-1}$] | $T$ [K] |
|---|---|---|---|---|---|---|---|
| 1a | 0.0 | 10.0 | 100.0 | 2a | 75.0 | 10.0 | 50.0 |
| 1b | 0.0 | 30.0 | 225.0 | 2b | 75.0 | 40.0 | 75.0 |
| 1c | 0.0 | 40.0 | 150.0 | 2c | 75.0 | 40.0 | 250.0 |
| 1d | 0.0 | 300.0 | 225.0 | 2d | 75.0 | 60.0 | 75.0 |
| 1e | 0.0 | 350.0 | 400.0 | 2e | 75.0 | 70.0 | 75.0 |
| 1f | 25.0 | 10.0 | 300.0 | 2f | 75.0 | 70.0 | 400.0 |
| 1g | 25.0 | 20.0 | 250.0 | 2g | 75.0 | 100.0 | 200.0 |
| 1h | 25.0 | 70.0 | 75.0 | 2h | 75.0 | 150.0 | 50.0 |
| 1i | 25.0 | 70.0 | 225.0 | 2i | 75.0 | 150.0 | 125.0 |
| 1j | 25.0 | 100.0 | 400.0 | 2j | 75.0 | 250.0 | 225.0 |
| 1k | 25.0 | 200.0 | 350.0 | 2k | 75.0 | 400.0 | 150.0 |
| 1l | 25.0 | 300.0 | 100.0 | 2l | 75.0 | 400.0 | 225.0 |
| 1m | 25.0 | 300.0 | 300.0 | 2m | 100.0 | 30.0 | 250.0 |
| 1n | 25.0 | 350.0 | 400.0 | 2n | 100.0 | 50.0 | 125.0 |
| 1o | 25.0 | 400.0 | 350.0 | 2o | 100.0 | 50.0 | 225.0 |
| 1p | 25.0 | 500.0 | 50.0 | 2p | 100.0 | 250.0 | 200.0 |
| 1q | 25.0 | 500.0 | 150.0 | 2q | 100.0 | 350.0 | 100.0 |
| 1r | 50.0 | 30.0 | 225.0 | 2r | 100.0 | 350.0 | 175.0 |
| 1s | 50.0 | 40.0 | 150.0 | 2s | 125.0 | 2.0 | 125.0 |
| 1t | 50.0 | 60.0 | 100.0 | 2t | 125.0 | 2.0 | 150.0 |
| 1u | 225.0 | 80.0 | 50.0 | 2u | 125.0 | 2.0 | 350.0 |
| 1v | 50.0 | 200.0 | 250.0 | 2v | 125.0 | 30.0 | 175.0 |
| 1x | 50.0 | 300.0 | 75.0 | 2x | 125.0 | 40.0 | 200.0 |
| 1y | 50.0 | 300.0 | 175.0 | 2y | 125.0 | 40.0 | 250.0 |
| 3a | 125.0 | 80.0 | 175.0 | 4a | 225.0 | 20.0 | 125.0 |
| 3b | 125.0 | 100.0 | 150.0 | 4b | 225.0 | 60.0 | 125.0 |
| 3c | 125.0 | 250.0 | 400.0 | 4c | 225.0 | 60.0 | 400.0 |
| 3d | 125.0 | 500.0 | 50.0 | 4d | 225.0 | 80.0 | 100.0 |
| 3e | 125.0 | 500.0 | 125.0 | 4e | 225.0 | 80.0 | 400.0 |
| 3f | 150.0 | 2.0 | 400.0 | 4f | 225.0 | 250.0 | 150.0 |
| 3g | 150.0 | 60.0 | 400.0 | 4g | 225.0 | 450.0 | 225.0 |
| 3h | 150.0 | 70.0 | 225.0 | 4h | 250.0 | 10.0 | 125.0 |
| 3i | 150.0 | 450.0 | 125.0 | 4i | 250.0 | 20.0 | 150.0 |
| 3j | 175.0 | 10.0 | 50.0 | 4j | 250.0 | 60.0 | 75.0 |
| 3k | 175.0 | 50.0 | 100.0 | 4k | 250.0 | 150.0 | 300.0 |
| 3l | 175.0 | 50.0 | 250.0 | 4l | 250.0 | 500.0 | 250.0 |
| 3m | 175.0 | 50.0 | 350.0 | 4m | 300.0 | 2.0 | 300.0 |
| 3n | 175.0 | 80.0 | 225.0 | 4n | 0.0 | 80.0 | 275.0 |
| 3o | 175.0 | 100.0 | 100.0 | 4o | 50.0 | 250.0 | 275.0 |
| 3p | 175.0 | 300.0 | 400.0 | 4p | 50.0 | 450.0 | 325.0 |
| 3q | 175.0 | 450.0 | 400.0 | 4q | 75.0 | 50.0 | 375.0 |
| 3r | 200.0 | 20.0 | 200.0 | 4r | 150.0 | 70.0 | 275.0 |
| 3s | 200.0 | 30.0 | 400.0 | 4s | 150.0 | 450.0 | 375.0 |
| 3t | 200.0 | 60.0 | 400.0 | 4t | 175.0 | 80.0 | 325.0 |
| 3u | 200.0 | 80.0 | 150.0 | 4u | 200.0 | 30.0 | 325.0 |
| 3v | 200.0 | 100.0 | 75.0 | 4v | 200.0 | 70.0 | 275.0 |
| 3x | 200.0 | 150.0 | 300.0 | 4x | 200.0 | 150.0 | 375.0 |
| 3y | 200.0 | 400.0 | 350.0 | 4y | 200.0 | 200.0 | 325.0 |
| 5a | 200.0 | 500.0 | 275.0 | 5m | 275.0 | 60.0 | 375.0 |
| 5b | 225.0 | 80.0 | 375.0 | 5n | 275.0 | 70.0 | 375.0 |
| 5c | 225.0 | 100.0 | 275.0 | 5o | 275.0 | 150.0 | 75.0 |
| 5d | 225.0 | 300.0 | 375.0 | 5p | 275.0 | 250.0 | 175.0 |
| 5e | 250.0 | 30.0 | 325.0 | 5q | 275.0 | 250.0 | 375.0 |
| 5f | 300.0 | 10.0 | 325.0 | 5r | 275.0 | 350.0 | 175.0 |
| 5g | 300.0 | 40.0 | 275.0 | 5s | 275.0 | 350.0 | 325.0 |
| 5h | 300.0 | 450.0 | 275.0 | 5t | 275.0 | 400.0 | 350.0 |
| 5i | 275.0 | 2.0 | 275.0 | 5u | 275.0 | 400.0 | 400.0 |
| 5j | 275.0 | 20.0 | 350.0 | 5v | 50.0 | 60.0 | 25.0 |
| 5k | 275.0 | 30.0 | 375.0 | 5x | 175.0 | 80.0 | 25.0 |
| 5l | 275.0 | 60.0 | 275.0 | 5y | 250.0 | 250.0 | 25.0 |

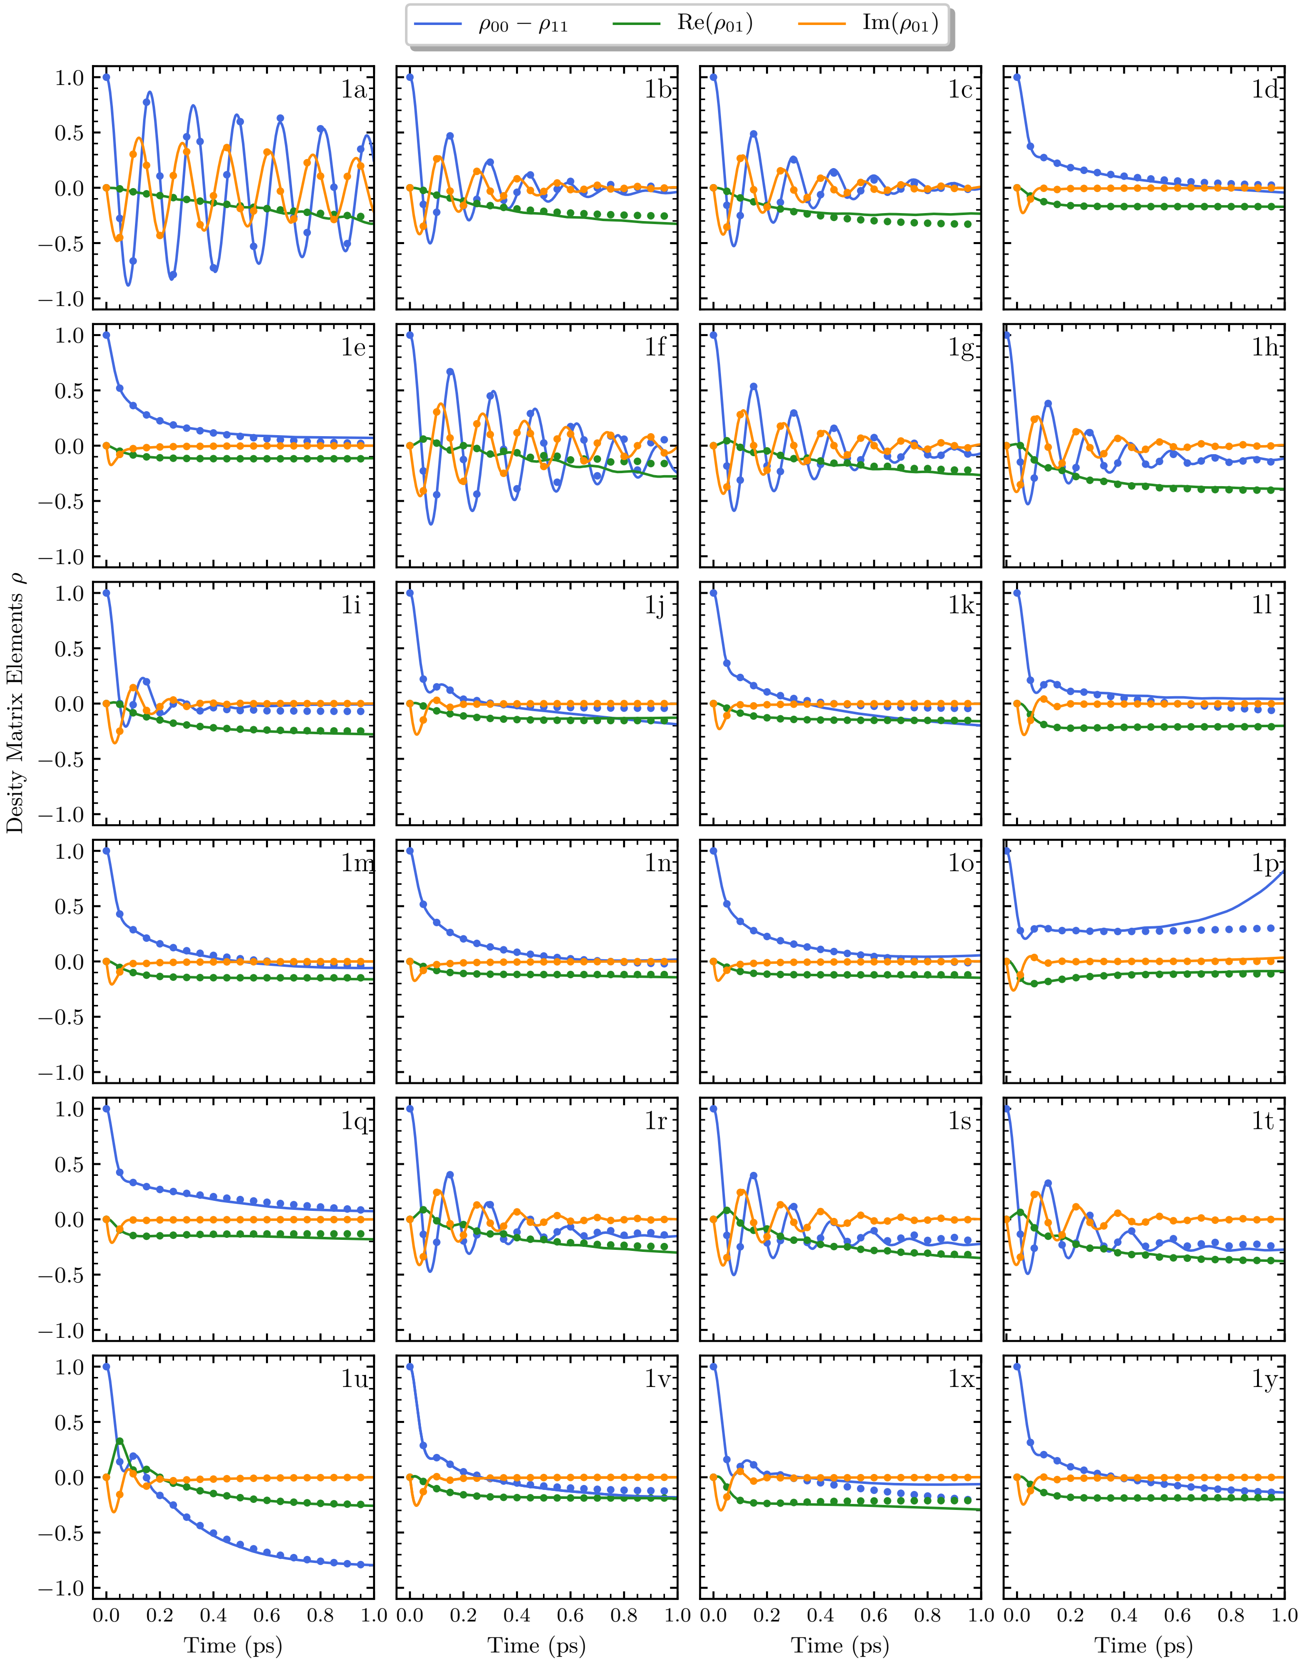


FIG. S1. Expectation value of $\hat{\sigma}_z$ as a function of time predicted by the artificial neural network model developed in this work (solid lines) for various sets of parameters compared to the exact results (circles) obtained with the HEOM method. The system and bath parameters corresponding to each plot are summarized in Table S1.

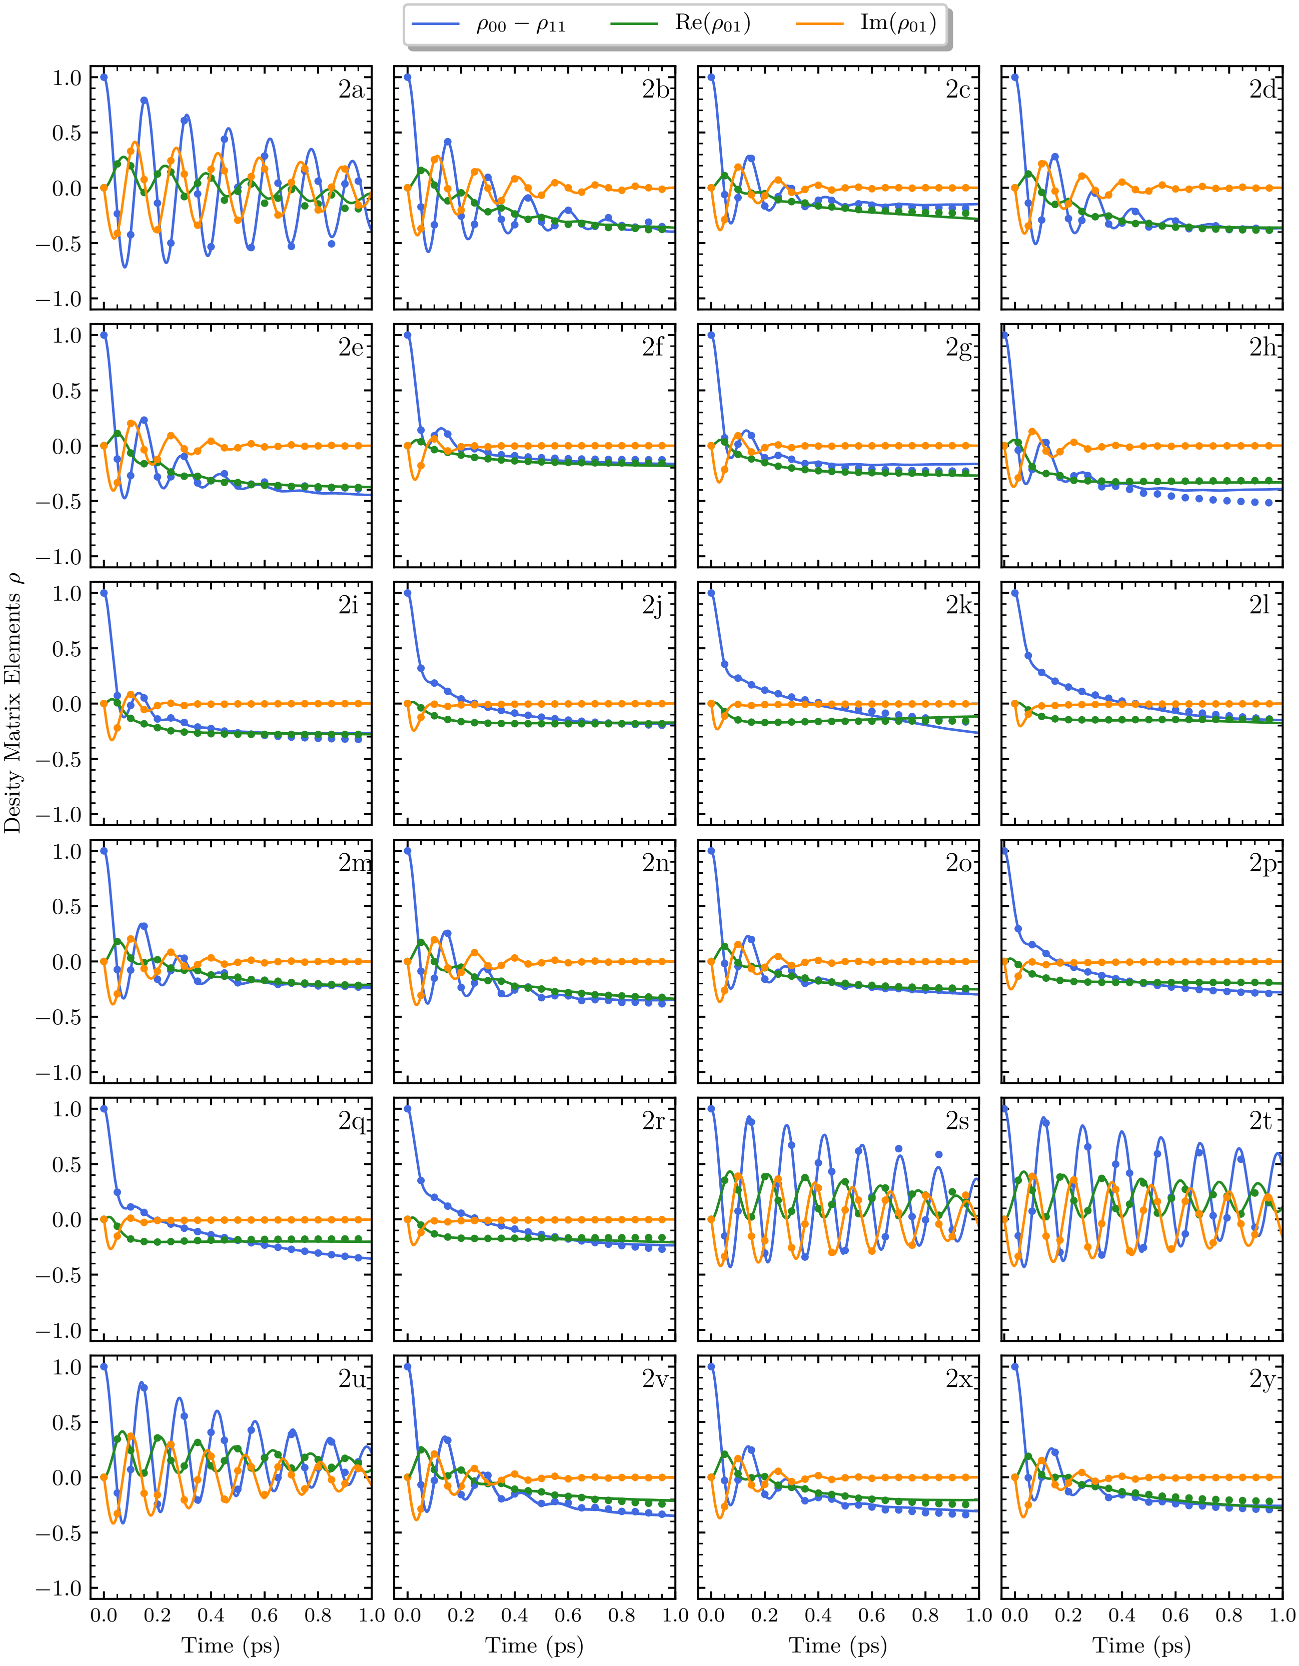


FIG. S2. Expectation value of $\hat{\sigma}_z$ as a function of time predicted by the artificial neural network model developed in this work (solid lines) for various sets of parameters compared to the exact results (circles) obtained with the HEOM method. The system and bath parameters corresponding to each plot are summarized in Table S1.

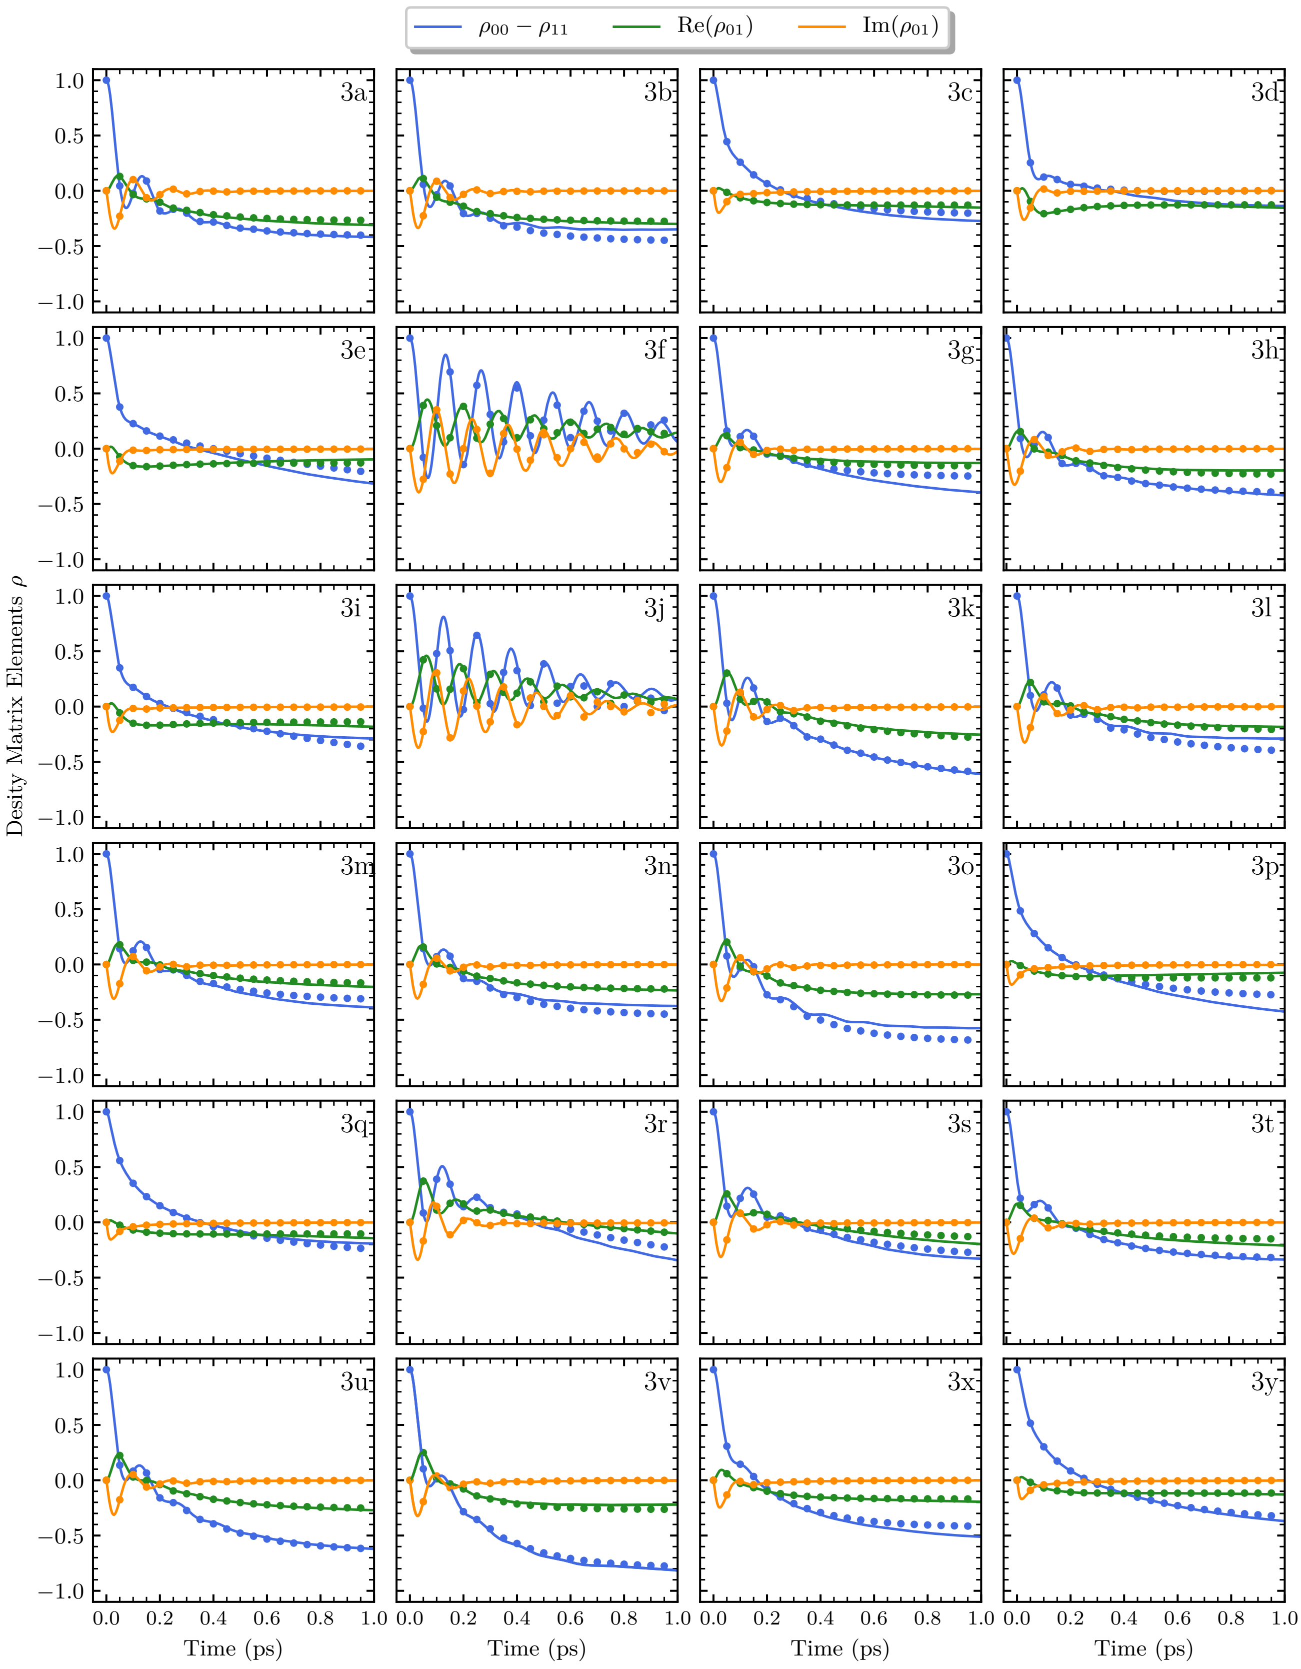


FIG. S3. Expectation value of $\hat{\sigma}_z$ as a function of time predicted by the artificial neural network model developed in this work (solid lines) for various sets of parameters compared to the exact results (circles) obtained with the HEOM method. The system and bath parameters corresponding to each plot are summarized in Table S1.

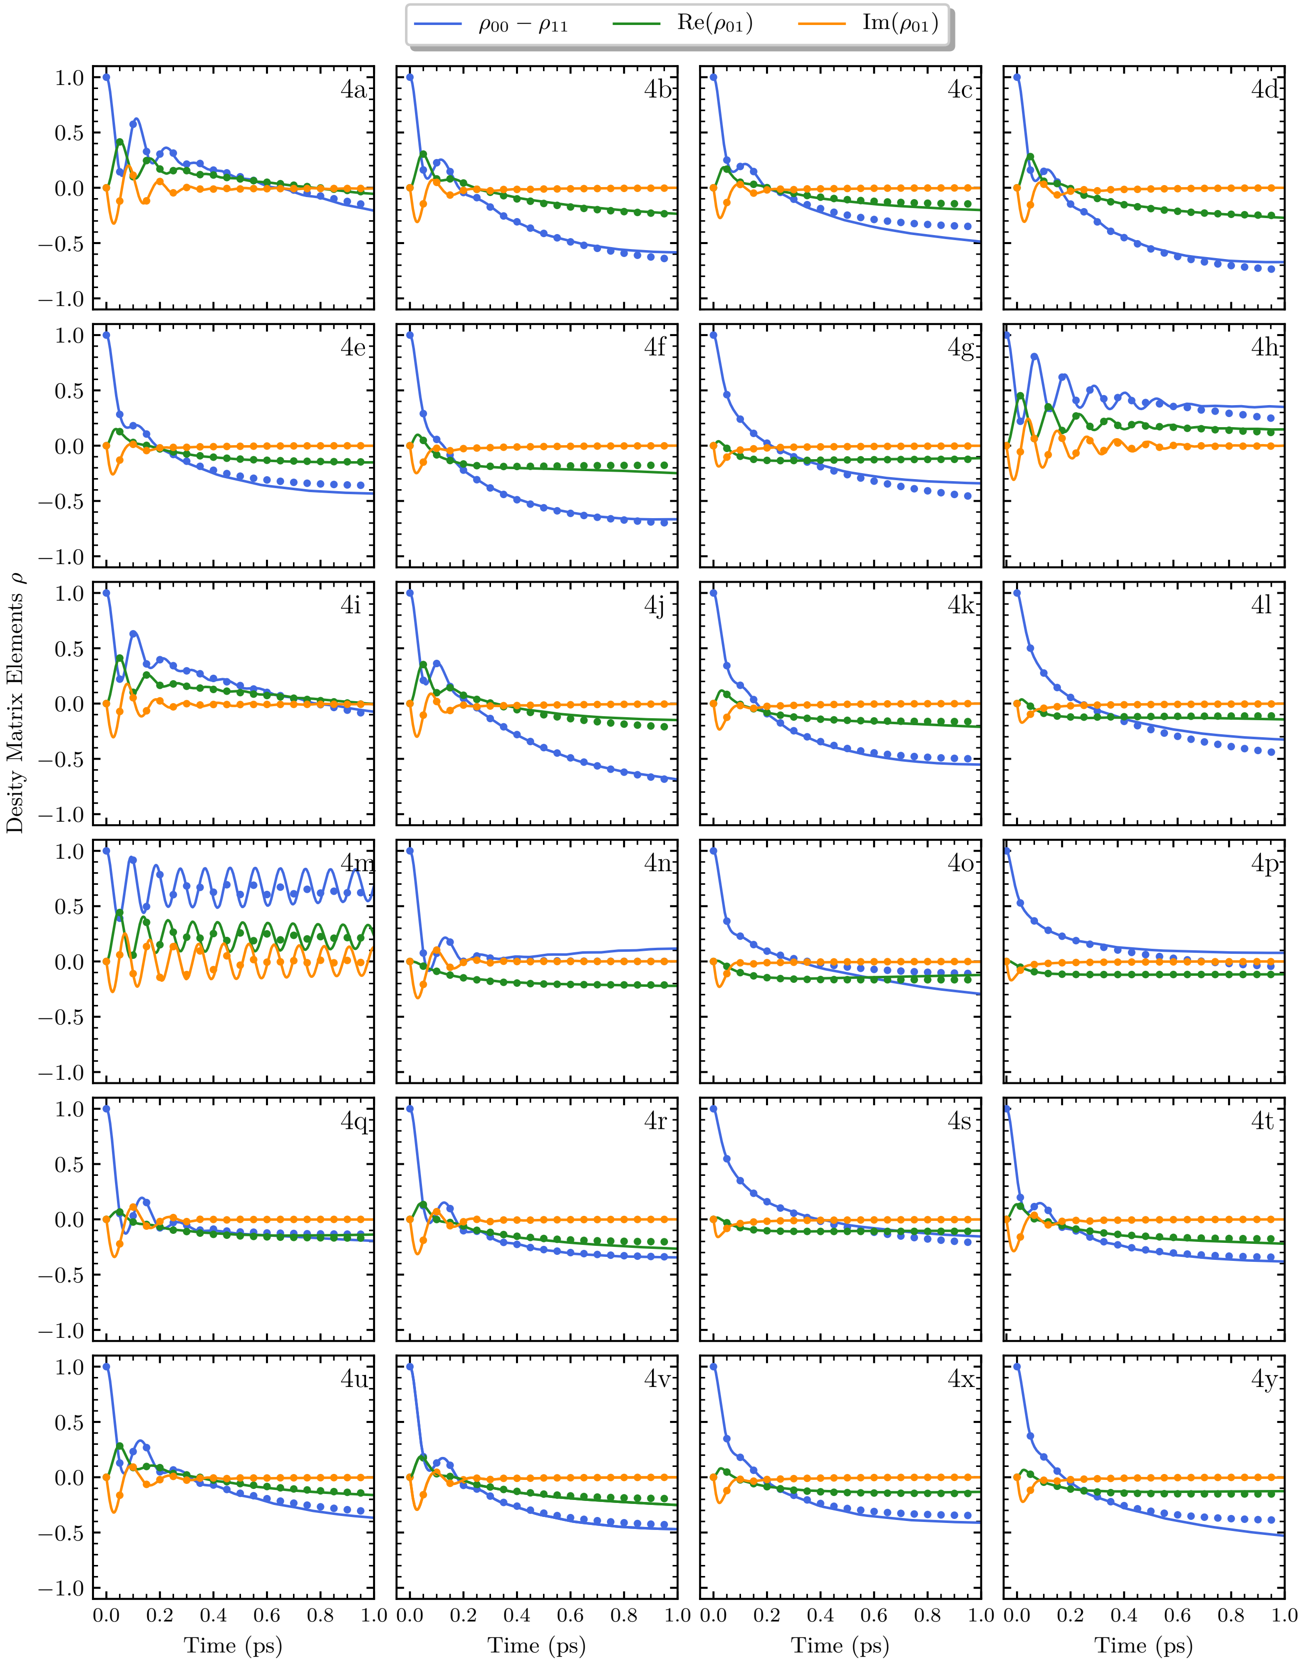


FIG. S4. Expectation value of $\hat{\sigma}_z$ as a function of time predicted by the artificial neural network model developed in this work (solid lines) for various sets of parameters compared to the exact results (circles) obtained with the HEOM method. The system and bath parameters corresponding to each plot are summarized in Table S1.

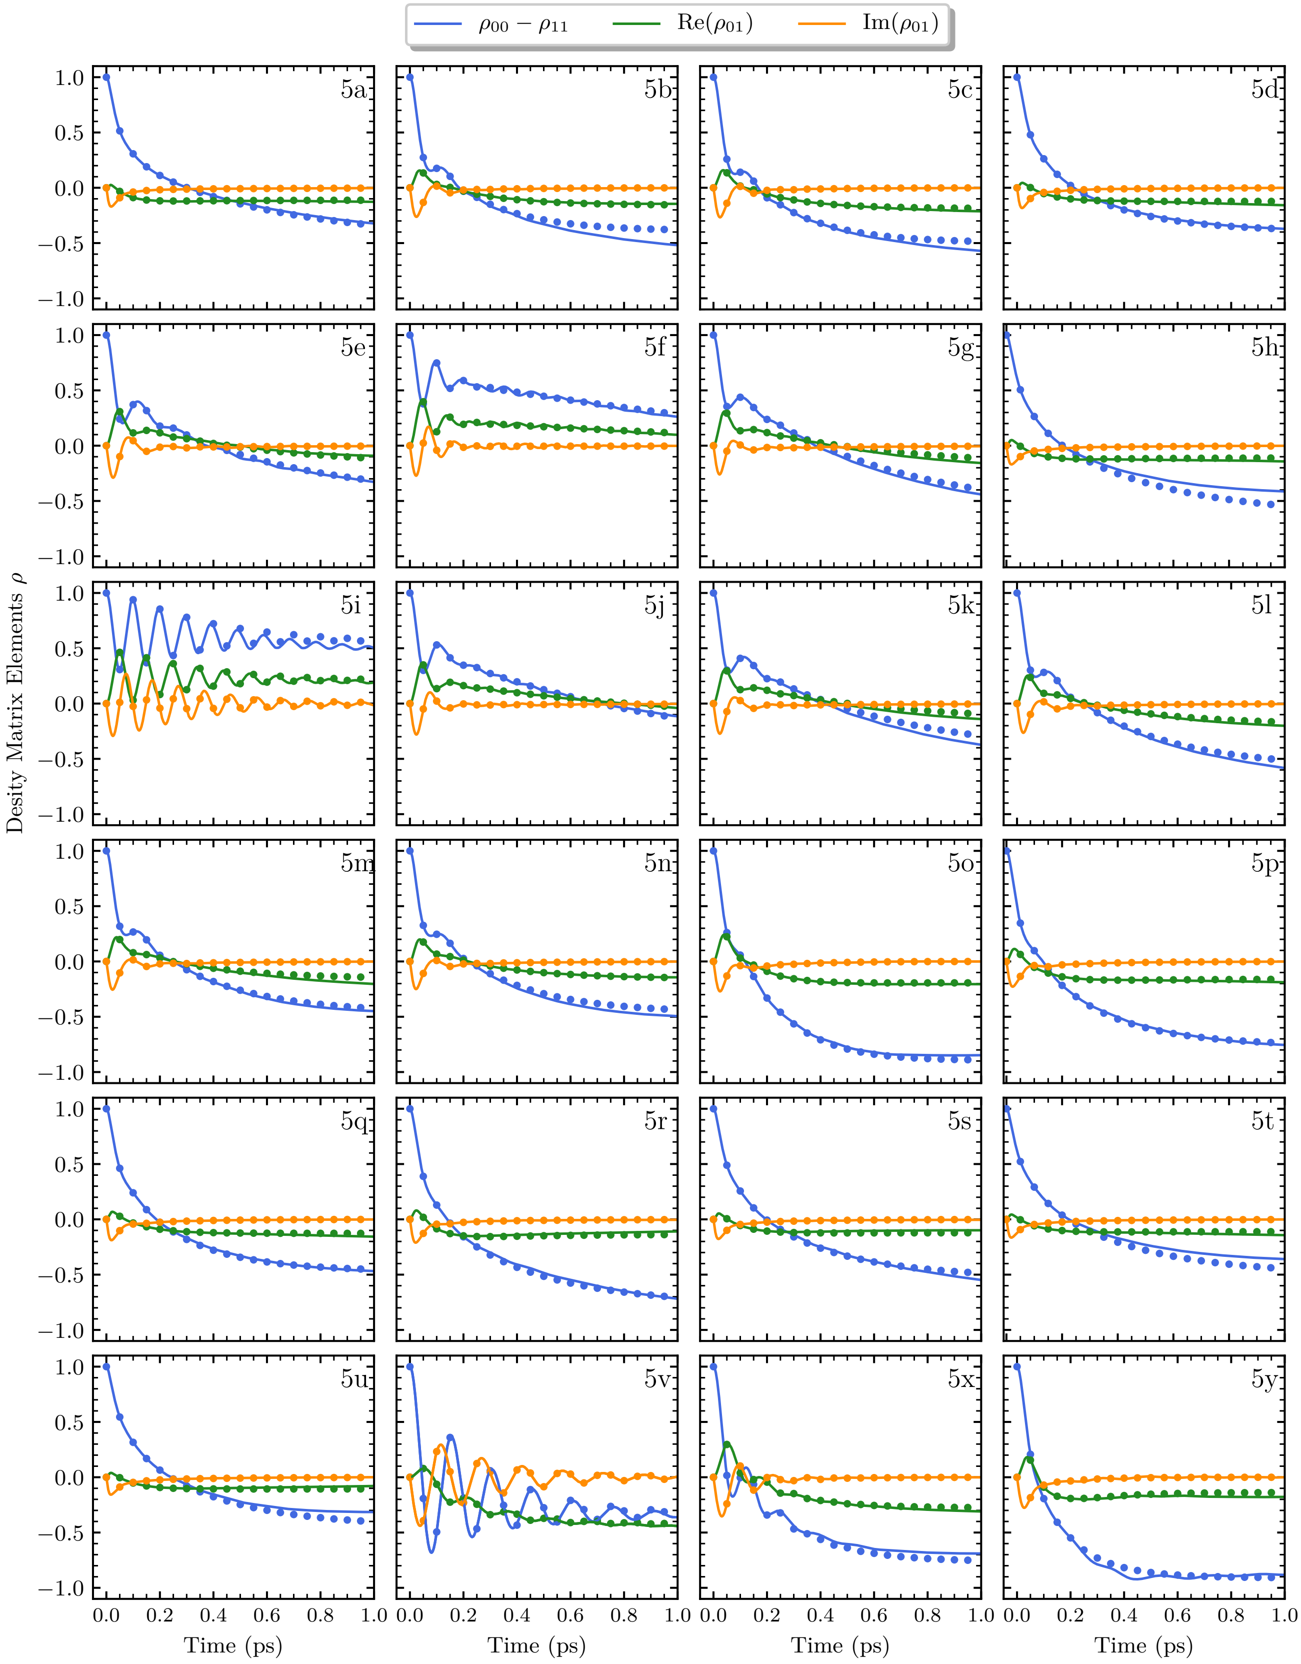


FIG. S5. Expectation value of $\hat{\sigma}_z$ as a function of time predicted by the artificial neural network model developed in this work (solid lines) for various sets of parameters compared to the exact results (circles) obtained with the HEOM method. The system and bath parameters corresponding to each plot are summarized in Table S1.

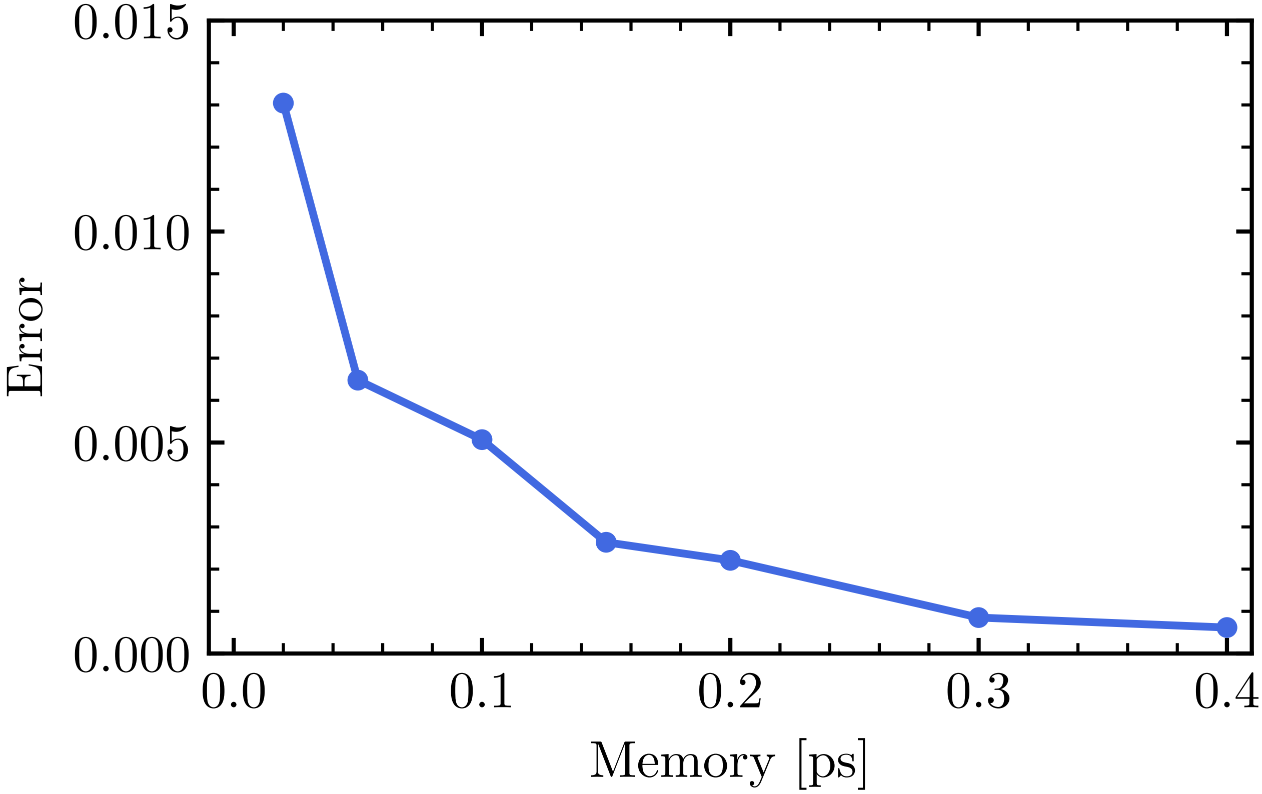


FIG. S6. The single time-step mean absolute errors (MAE) of the predicted RDMs with respect to the memory time. A set of 150 combinations of system and bath parameters randomly chosen from the total data set was used. For each set the reduced density matrix was propagated by the ANN model developed in this work up to 1.0 ps starting from the initial 0.2 ps long HEOM trajectory.
